# Supplementary material for: Observational evidence for bar formation in disk galaxies via cluster-cluster interaction
Source: arXiv:1906.10585 source file (2019-06-25)
Supplement: Supplementary file 1 [file bar_supplement.pdf]

Observational evidence for bar formation in disk galaxies via cluster-cluster interaction
(Supplementary information)

Yongmin Yoon,[1] Myungshin Im,[1] Gwang-Ho Lee,[2,3] Seong-Kook Lee,[1] and Gu Lim[1]

[1] *Center for the Exploration of the Origin of the Universe (CEOU), Astronomy Program, Department of Physics and Astronomy, Seoul National University, 1 Gwanak-ro, Gwanak-gu, Seoul, 151-742, Republic of Korea*

[2] *Steward Observatory, University of Arizona, 933 North Cherry Avenue, Tucson, AZ 85721, USA*

[3] *Korea Astronomy and Space Science Institute, Daejeon 305-348, Republic of Korea*

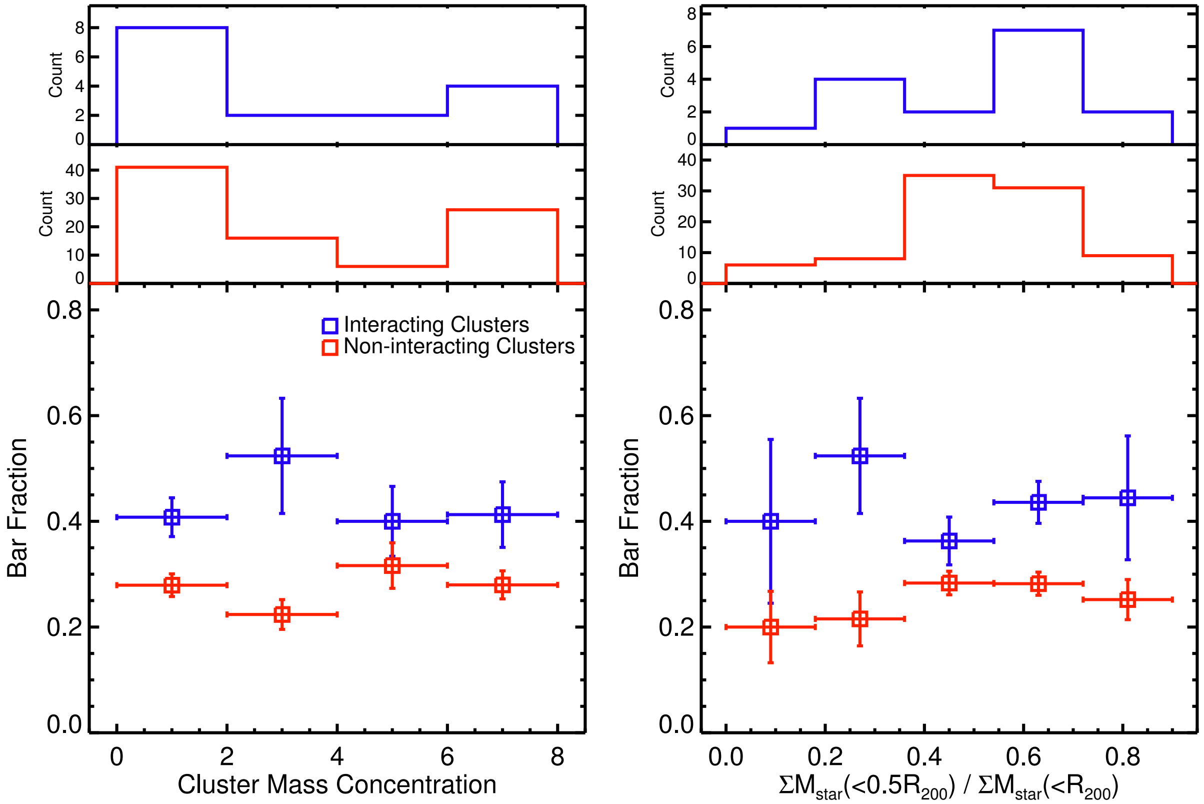


**Supplementary Figure 1. Bar fractions of disk-dominated galaxies in the interacting clusters and non-interacting clusters as a function of cluster mass concentrations with distributions for the number of galaxies contained in each bin.** In the left panel, we used cluster mass concentrations, which were derived by fitting the projected Navarro–Frenk–White (NFW) profiles to the surface stellar mass density distributions of the member galaxies in clusters. This method has been used in several previous studies[1,2,3], in which they found that cluster stellar mass profiles are similar to the cluster dark matter profiles and well described by the NFW profile, but with slightly lower concentration values compared to those of estimated dark matter profiles. The highest concentration bin in the left panel includes clusters with concentration values larger than 8. In the right panel, we used another proxy for the cluster mass concentration, which was defined as the total stellar mass within a half of $R_{200}$ divided by the total stellar mass within $R_{200}$. We conclude that the bar fraction is not dependent on the cluster mass concentration.

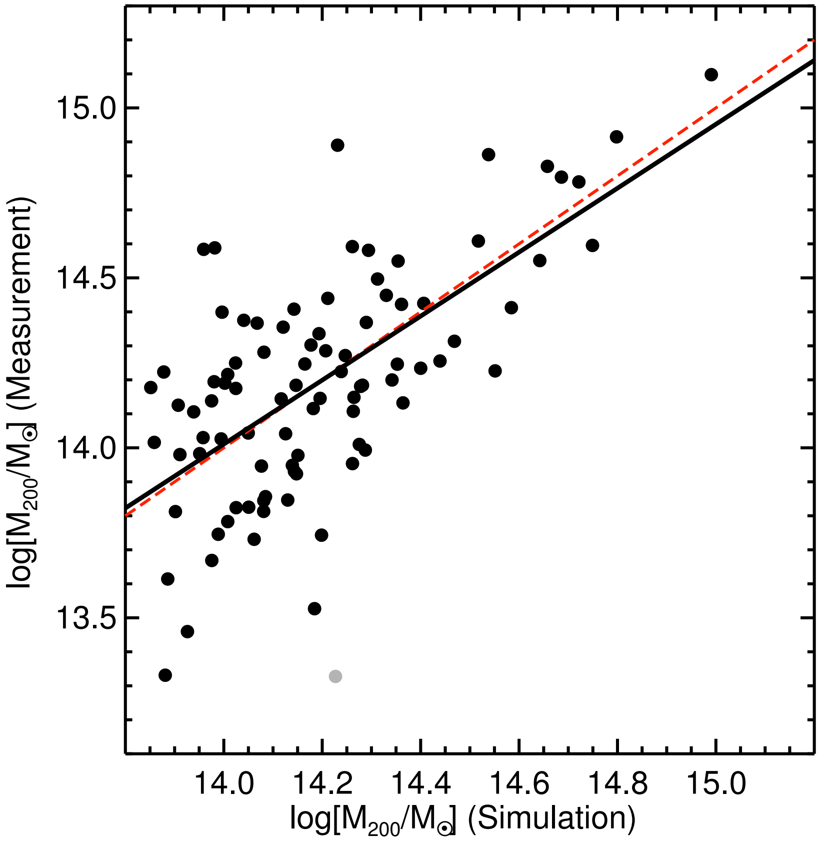


**Supplementary Figure 2. Comparison between $M_{200}$ from the simulation and $M_{200}$ measured by our method.** The gray point indicates one outlier beyond $\pm 3\sigma$. The black solid line is the best-fit line for data except the outlier. The red dashed line denotes the equal quantity for the both values.

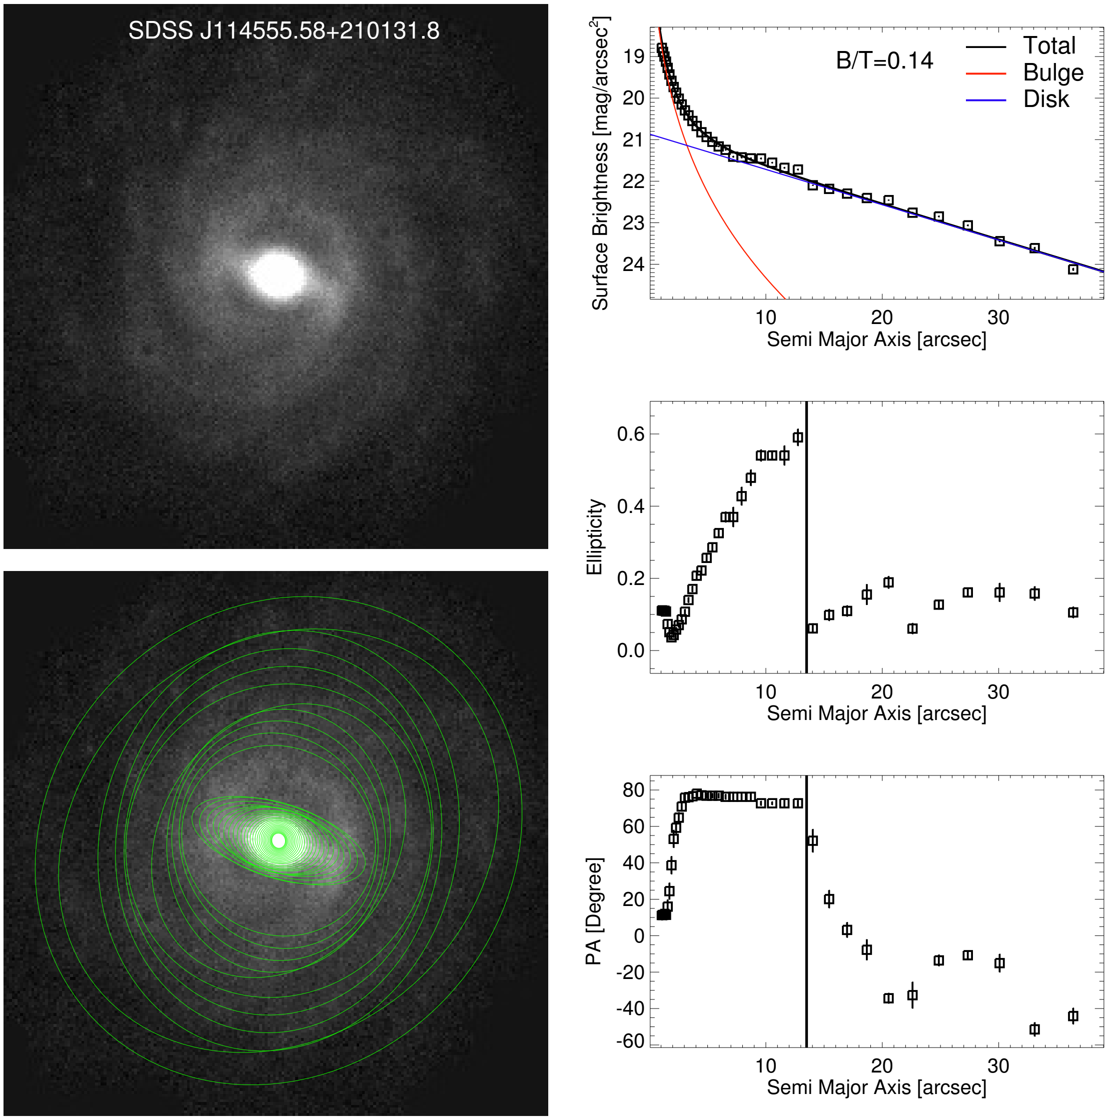


**Supplementary Figure 3. Typical example of barred galaxy with the fitted ellipses on the image.** The surface brightness profile and the fitted model profiles are at the top of the right panel. The ellipticity profile and the position angle profile are also shown at the middle and the bottom of the right panel, respectively. The vertical solid lines indicate the transition semi-major axis where sudden changes in the ellipticity and position angle are observed.

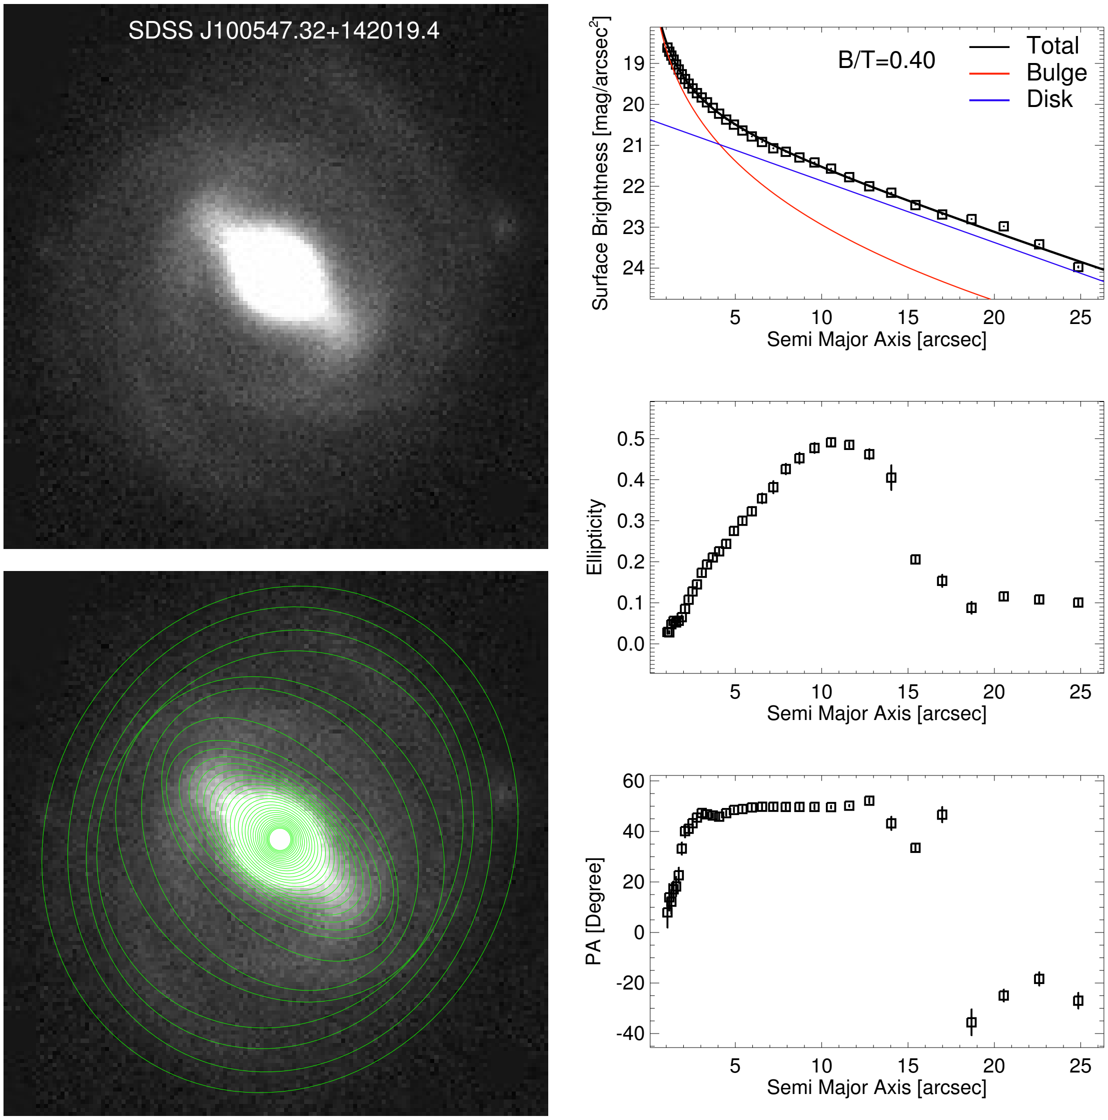


**Supplementary Figure 4. Typical example of barred galaxy with the fitted ellipses on the image.** The surface brightness profile and the fitted model profiles are at the top of the right panel. The ellipticity profile and the position angle profile are also shown at the middle and the bottom of the right panel, respectively.

**Supplementary Table 1**. Properties of Galaxy Clusters

| Name | RA | Dec | Redshift | $\sigma_v$ [km s$^{-1}$] | $R_{200}$ [Mpc] | $\log(M_{200}/M_{\odot})$ | $\log p$ | Interacting | $f_{\rm bar}$(bar/disk) |
|---|---|---|---|---|---|---|---|---|---|
| (1) | (2) | (3) | (4) | (5) | (6) | (7) | (8) | (9) | (10) |
| Cluster0029−00 | 7.31126 | -0.18845 | 0.05947 | $450 \pm 49$ | $1.1 \pm 0.1$ | $14.2 \pm 0.1$ | -1.26 | N | 0.462 (6/13) |
| Cluster0041−09 | 10.39558 | -9.36069 | 0.05701 | $691 \pm 50$ | $1.7 \pm 0.1$ | $14.7 \pm 0.1$ | -0.53 | N | 0.125 (2/16) |
| Cluster0056−10 | 14.07577 | -10.09807 | 0.05494 | $504 \pm 37$ | $1.2 \pm 0.1$ | $14.3 \pm 0.1$ | -0.06 | N | 0.455 (5/11) |
| Cluster0056−00 | 14.09811 | -0.98688 | 0.04403 | $877 \pm 75$ | $2.1 \pm 0.2$ | $15.1 \pm 0.1$ | -1.79 | N | 0.324 (11/34) |
| Cluster0110+14 | 17.53863 | 14.12326 | 0.05881 | $688 \pm 70$ | $1.7 \pm 0.2$ | $14.7 \pm 0.1$ | -0.85 | N | 0.214 (3/14) |
| Cluster0112+15 | 18.24815 | 15.49130 | 0.04385 | $750 \pm 88$ | $1.8 \pm 0.2$ | $14.9 \pm 0.2$ | -0.56 | N | 0.333 (5/15) |
| Cluster0114+00 | 18.63715 | 0.23377 | 0.04494 | $514 \pm 48$ | $1.2 \pm 0.1$ | $14.4 \pm 0.1$ | -0.30 | N | 0.360 (9/25) |
| Cluster0137−09 | 24.36158 | -9.21754 | 0.03897 | $543 \pm 77$ | $1.3 \pm 0.2$ | $14.4 \pm 0.2$ | -0.13 | N | 0.333 (4/12) |
| Cluster0319+41 | 49.93559 | 41.27807 | 0.01836 | $1006 \pm 80$ | $2.5 \pm 0.2$ | $15.2 \pm 0.1$ | -0.85 | N | 0.185 (5/27) |
| Cluster0325−00 | 51.32768 | -0.63158 | 0.03603 | $365 \pm 67$ | $0.9 \pm 0.2$ | $13.9 \pm 0.3$ | -0.77 | N | 0.000 (0/4) |
| Cluster0745+18 | 116.40416 | 18.25487 | 0.05080 | $631 \pm 87$ | $1.5 \pm 0.2$ | $14.6 \pm 0.2$ | -0.19 | N | 0.143 (2/14) |
| Cluster0748+18 | 117.09089 | 18.54871 | 0.04777 | $570 \pm 55$ | $1.4 \pm 0.1$ | $14.5 \pm 0.1$ | -0.07 | N | 0.222 (4/18) |
| Cluster0755+45 | 118.85122 | 45.84683 | 0.05242 | $508 \pm 86$ | $1.2 \pm 0.2$ | $14.3 \pm 0.2$ | -0.03 | N | 0.222 (2/9) |
| Cluster0758+37 | 119.61712 | 37.78657 | 0.04082 | $381 \pm 62$ | $0.9 \pm 0.2$ | $14.0 \pm 0.2$ | -0.33 | N | 0.200 (1/5) |
| Cluster0828+30 | 127.21100 | 30.59652 | 0.04999 | $832 \pm 68$ | $2.0 \pm 0.2$ | $15.0 \pm 0.1$ | -1.66 | N | 0.182 (4/22) |
| Cluster0835+38 | 128.95018 | 38.55400 | 0.05591 | $393 \pm 48$ | $0.9 \pm 0.1$ | $14.0 \pm 0.2$ | -1.34 | N | 0.143 (1/7) |
| Cluster0842+36 | 130.62154 | 36.11389 | 0.05378 | $436 \pm 61$ | $1.1 \pm 0.1$ | $14.1 \pm 0.2$ | -1.21 | N | 0.429 (3/7) |
| Cluster0847+53 | 131.90311 | 53.76255 | 0.04398 | $446 \pm 60$ | $1.1 \pm 0.1$ | $14.2 \pm 0.2$ | -0.55 | N | 0.250 (1/4) |
| Cluster0913+47 | 138.33553 | 47.71940 | 0.05176 | $351 \pm 38$ | $0.8 \pm 0.1$ | $13.9 \pm 0.2$ | -0.06 | N | 0.250 (2/8) |
| Cluster0916+17 | 139.04343 | 17.52184 | 0.02890 | $423 \pm 69$ | $1.0 \pm 0.2$ | $14.1 \pm 0.2$ | -1.77 | N | 0.571 (4/7) |
| Cluster0917+20 | 139.36517 | 20.23475 | 0.03024 | $468 \pm 70$ | $1.1 \pm 0.2$ | $14.2 \pm 0.2$ | -0.79 | N | 0.500 (5/10) |
| Cluster0919+33 | 139.96790 | 33.64950 | 0.02223 | $616 \pm 97$ | $1.5 \pm 0.2$ | $14.6 \pm 0.2$ | -0.73 | N | 0.333 (3/9) |
| Cluster0923+22 | 140.87479 | 22.32714 | 0.03067 | $608 \pm 104$ | $1.5 \pm 0.3$ | $14.6 \pm 0.2$ | -0.14 | N | 0.375 (3/8) |
| Cluster0946+54 | 146.62085 | 54.64478 | 0.04653 | $507 \pm 53$ | $1.2 \pm 0.1$ | $14.3 \pm 0.1$ | -0.72 | N | 0.083 (1/12) |
| Cluster1001+32 | 150.49860 | 32.79404 | 0.05088 | $393 \pm 46$ | $1.0 \pm 0.1$ | $14.0 \pm 0.2$ | -0.12 | N | 0.167 (1/6) |
| Cluster1004+54 | 151.06337 | 54.66267 | 0.04731 | $454 \pm 72$ | $1.1 \pm 0.2$ | $14.2 \pm 0.2$ | -0.79 | Y: Pair | 0.556 (5/9) |
| Cluster1006+14 | 151.71735 | 14.37584 | 0.03030 | $355 \pm 44$ | $0.9 \pm 0.1$ | $13.9 \pm 0.2$ | -0.47 | N | 0.600 (3/5) |
| Cluster1009+54 | 152.42709 | 54.47901 | 0.04546 | $364 \pm 58$ | $0.9 \pm 0.1$ | $13.9 \pm 0.2$ | -0.18 | Y: Pair | 0.400 (2/5) |
| Cluster1014−00 | 153.54002 | -0.86836 | 0.04597 | $746 \pm 53$ | $1.8 \pm 0.1$ | $14.8 \pm 0.1$ | -0.91 | N | 0.182 (2/11) |
| Cluster1021+23 | 155.36665 | 23.98188 | 0.03833 | $489 \pm 61$ | $1.2 \pm 0.2$ | $14.3 \pm 0.2$ | -1.45 | N | 0.333 (3/9) |
| Cluster1022+38 | 155.53812 | 38.51323 | 0.05409 | $731 \pm 79$ | $1.8 \pm 0.2$ | $14.8 \pm 0.1$ | -0.88 | N | 0.286 (4/14) |
| Cluster1032+56 | 158.15845 | 56.81041 | 0.04610 | $392 \pm 47$ | $1.0 \pm 0.1$ | $14.0 \pm 0.2$ | -0.03 | N | 0.143 (1/7) |
| Cluster1048+22 | 162.01007 | 22.37302 | 0.04618 | $415 \pm 61$ | $1.0 \pm 0.2$ | $14.1 \pm 0.2$ | -0.89 | N | 0.333 (2/6) |
| Cluster1058+01 | 164.66180 | 1.66207 | 0.03791 | $396 \pm 59$ | $1.0 \pm 0.1$ | $14.0 \pm 0.2$ | -0.88 | N | 0.333 (2/6) |
| Cluster1108+44 | 167.13342 | 44.09607 | 0.05938 | $585 \pm 49$ | $1.4 \pm 0.1$ | $14.5 \pm 0.1$ | -0.60 | N | 0.235 (4/17) |
| Cluster1110+28 | 167.67744 | 28.45831 | 0.03265 | $747 \pm 58$ | $1.8 \pm 0.1$ | $14.9 \pm 0.1$ | -5.00 | Y: Substructure | 0.348 (8/23) |
| Cluster1112+57 | 168.06956 | 57.07600 | 0.04714 | $466 \pm 65$ | $1.1 \pm 0.2$ | $14.2 \pm 0.2$ | -0.13 | N | 0.091 (1/11) |
| Cluster1114+25 | 168.73567 | 25.87285 | 0.04716 | $408 \pm 40$ | $1.0 \pm 0.1$ | $14.1 \pm 0.1$ | -0.01 | N | 0.375 (3/8) |
| Cluster1115+29 | 168.98116 | 29.30567 | 0.04706 | $533 \pm 54$ | $1.3 \pm 0.1$ | $14.4 \pm 0.1$ | -0.53 | N | 0.261 (6/23) |
| Cluster1121+02 | 170.42026 | 2.89833 | 0.04874 | $581 \pm 55$ | $1.4 \pm 0.1$ | $14.5 \pm 0.1$ | -0.22 | N | 0.250 (3/12) |
| Cluster1132+55[a] | 173.11852 | 55.99677 | 0.05531 | $1021 \pm 81$ | $2.5 \pm 0.2$ | $15.3 \pm 0.1$ | -1.90 | N | 0.214 (6/28) |
| Cluster1134+48 | 173.61664 | 48.96341 | 0.03396 | $585 \pm 65$ | $1.4 \pm 0.2$ | $14.5 \pm 0.2$ | -0.10 | N | 0.400 (4/10) |
| Cluster1136+55 | 174.03810 | 55.00997 | 0.05504 | $377 \pm 30$ | $0.9 \pm 0.1$ | $14.0 \pm 0.1$ | -0.25 | N | 0.200 (2/10) |
| Cluster1139+55 | 174.78896 | 55.61960 | 0.05994 | $393 \pm 45$ | $0.9 \pm 0.1$ | $14.0 \pm 0.2$ | -0.23 | N | 0.333 (3/9) |
| Cluster1144+19 | 176.08510 | 19.98086 | 0.02111 | $764 \pm 64$ | $1.9 \pm 0.2$ | $14.9 \pm 0.1$ | -1.61 | Y: Pair | 0.375 (9/24) |
| Cluster1148+54 | 177.07797 | 54.72366 | 0.05840 | $475 \pm 49$ | $1.1 \pm 0.1$ | $14.3 \pm 0.1$ | -0.14 | N | 0.417 (5/12) |
| Cluster1148+55 | 177.08051 | 55.81400 | 0.05121 | $653 \pm 71$ | $1.6 \pm 0.2$ | $14.7 \pm 0.1$ | -0.45 | N | 0.250 (5/20) |
| Cluster1151+21 | 177.92720 | 21.00273 | 0.02351 | $557 \pm 70$ | $1.4 \pm 0.2$ | $14.5 \pm 0.2$ | -0.99 | Y: Pair | 0.600 (6/10) |
| Cluster1204+20 | 181.00415 | 20.33742 | 0.02275 | $397 \pm 41$ | $1.0 \pm 0.1$ | $14.0 \pm 0.1$ | -0.25 | N | 0.154 (2/13) |
| Cluster1205+02 | 181.33980 | 2.08631 | 0.02176 | $564 \pm 90$ | $1.4 \pm 0.2$ | $14.5 \pm 0.2$ | -0.26 | N | 0.286 (2/7) |

*Supplementary Table 1 continued on next page*

**Supplementary Table 1** *(continued)*

| Name | RA | Dec | Redshift | $\sigma_v$ [km s$^{-1}$] | $R_{200}$ [Mpc] | $\log(M_{200}/M_{\odot})$ | $\log p$ | Interacting | $f_{\rm bar}$(bar/disk) |
|---|---|---|---|---|---|---|---|---|---|
| (1) | (2) | (3) | (4) | (5) | (6) | (7) | (8) | (9) | (10) |
| Cluster1206+28 | 181.52461 | 28.23804 | 0.02734 | $459 \pm 53$ | $1.1 \pm 0.1$ | $14.2 \pm 0.2$ | -0.16 | N | 0.111 (1/9) |
| Cluster1208+25 | 182.02315 | 25.23732 | 0.02253 | $355 \pm 57$ | $0.9 \pm 0.1$ | $13.9 \pm 0.2$ | -0.26 | N | 0.333 (2/6) |
| Cluster1219+28 | 184.97255 | 28.38586 | 0.02650 | $360 \pm 30$ | $0.9 \pm 0.1$ | $13.9 \pm 0.1$ | -0.66 | N | 0.667 (4/6) |
| Cluster1259+27 | 194.78416 | 27.78413 | 0.02345 | $990 \pm 68$ | $2.4 \pm 0.2$ | $15.2 \pm 0.1$ | -1.11 | N | 0.368 (25/68) |
| Cluster1306+43 | 196.68353 | 43.65523 | 0.03731 | $454 \pm 46$ | $1.1 \pm 0.1$ | $14.2 \pm 0.1$ | -1.02 | N | 0.400 (2/5) |
| Cluster1316+07 | 199.11505 | 7.03511 | 0.05056 | $556 \pm 71$ | $1.3 \pm 0.2$ | $14.5 \pm 0.2$ | -0.71 | N | 0.286 (4/14) |
| Cluster1321+33 | 200.30476 | 33.07927 | 0.03711 | $429 \pm 50$ | $1.0 \pm 0.1$ | $14.1 \pm 0.2$ | -0.61 | N | 0.333 (2/6) |
| Cluster1325+08 | 201.32014 | 8.32901 | 0.05116 | $367 \pm 45$ | $0.9 \pm 0.1$ | $13.9 \pm 0.2$ | -0.12 | N | 0.200 (1/5) |
| Cluster1329+37 | 202.37703 | 37.52594 | 0.05614 | $572 \pm 64$ | $1.4 \pm 0.2$ | $14.5 \pm 0.2$ | -0.67 | N | 0.250 (4/16) |
| Cluster1336+35 | 204.13858 | 35.98060 | 0.05922 | $434 \pm 50$ | $1.0 \pm 0.1$ | $14.1 \pm 0.2$ | -4.40 | Y: Substructure | 0.400 (4/10) |
| Cluster1342+29 | 205.71268 | 29.83242 | 0.04370 | $723 \pm 96$ | $1.8 \pm 0.2$ | $14.8 \pm 0.2$ | -0.29 | N | 0.333 (2/6) |
| Cluster1348+25 | 207.09320 | 25.68049 | 0.05140 | $443 \pm 65$ | $1.1 \pm 0.2$ | $14.2 \pm 0.2$ | -0.39 | N | 0.286 (2/7) |
| Cluster1410+19 | 212.73271 | 19.03392 | 0.05675 | $378 \pm 41$ | $0.9 \pm 0.1$ | $14.0 \pm 0.1$ | -0.58 | N | 0.000 (0/4) |
| Cluster1417+02 | 214.38362 | 2.17981 | 0.05270 | $592 \pm 60$ | $1.4 \pm 0.1$ | $14.5 \pm 0.1$ | -0.15 | N | 0.250 (3/12) |
| Cluster1417+00 | 214.46359 | 0.31953 | 0.05264 | $486 \pm 76$ | $1.2 \pm 0.2$ | $14.3 \pm 0.2$ | -0.62 | N | 0.286 (2/7) |
| Cluster1417+08 | 214.48317 | 8.21171 | 0.05795 | $557 \pm 61$ | $1.3 \pm 0.1$ | $14.5 \pm 0.1$ | -0.61 | N | 0.364 (4/11) |
| Cluster1426+16 | 216.71732 | 16.75641 | 0.05355 | $567 \pm 58$ | $1.4 \pm 0.1$ | $14.5 \pm 0.1$ | -2.33 | N | 0.190 (4/21) |
| Cluster1431−01 | 217.75015 | -1.80042 | 0.05389 | $424 \pm 51$ | $1.0 \pm 0.1$ | $14.1 \pm 0.2$ | -1.78 | N | 0.333 (2/6) |
| Cluster1440+03 | 220.16257 | 3.46972 | 0.02665 | $382 \pm 49$ | $0.9 \pm 0.1$ | $14.0 \pm 0.2$ | -0.11 | N | 0.167 (2/12) |
| Cluster1449+11 | 222.37593 | 11.24766 | 0.05055 | $507 \pm 80$ | $1.2 \pm 0.2$ | $14.3 \pm 0.2$ | -1.64 | N | 0.300 (3/10) |
| Cluster1453+16 | 223.30621 | 16.93537 | 0.04531 | $474 \pm 38$ | $1.2 \pm 0.1$ | $14.3 \pm 0.1$ | -1.87 | N | 0.308 (4/13) |
| Cluster1454+18 | 223.61671 | 18.61569 | 0.05886 | $534 \pm 48$ | $1.3 \pm 0.1$ | $14.4 \pm 0.1$ | -2.54 | N | 0.143 (2/14) |
| Cluster1504+28 | 226.14388 | 28.47159 | 0.05909 | $669 \pm 58$ | $1.6 \pm 0.1$ | $14.7 \pm 0.1$ | -0.04 | N | 0.118 (2/17) |
| Cluster1512+07 | 228.11340 | 7.36233 | 0.04555 | $623 \pm 54$ | $1.5 \pm 0.1$ | $14.6 \pm 0.1$ | -1.85 | N | 0.286 (4/14) |
| Cluster1516+07 | 229.07976 | 7.16234 | 0.03603 | $639 \pm 69$ | $1.6 \pm 0.2$ | $14.6 \pm 0.1$ | -0.76 | Y: Pair | 0.500 (7/14) |
| Cluster1518+04 | 229.55058 | 4.52199 | 0.03577 | $424 \pm 74$ | $1.0 \pm 0.2$ | $14.1 \pm 0.2$ | -0.29 | N | 0.100 (1/10) |
| Cluster1519+20 | 229.81667 | 20.79052 | 0.03994 | $399 \pm 43$ | $1.0 \pm 0.1$ | $14.0 \pm 0.1$ | -0.05 | Y: Pair | 0.571 (4/7) |
| Cluster1521+07 | 230.35884 | 7.72844 | 0.04515 | $543 \pm 58$ | $1.3 \pm 0.1$ | $14.4 \pm 0.1$ | -0.01 | N | 0.500 (8/16) |
| Cluster1523+08 | 230.79326 | 8.50535 | 0.03587 | $798 \pm 66$ | $1.9 \pm 0.2$ | $14.9 \pm 0.1$ | -0.83 | Y: Pair | 0.429 (9/21) |
| Cluster1523+20 | 230.93633 | 20.72727 | 0.04012 | $347 \pm 39$ | $0.8 \pm 0.1$ | $13.9 \pm 0.2$ | -0.43 | Y: Pair | 0.333 (1/3) |
| Cluster1532+04 | 233.14902 | 4.74245 | 0.03871 | $390 \pm 64$ | $0.9 \pm 0.2$ | $14.0 \pm 0.2$ | -0.46 | N | 0.000 (0/4) |
| Cluster1539+21 | 234.89738 | 21.74053 | 0.04160 | $564 \pm 49$ | $1.4 \pm 0.1$ | $14.5 \pm 0.1$ | -2.65 | N | 0.143 (2/14) |
| Cluster1551+34 | 237.94614 | 34.05005 | 0.04958 | $504 \pm 84$ | $1.2 \pm 0.2$ | $14.3 \pm 0.3$ | -2.86 | N | 0.556 (5/9) |
| Cluster1557+20 | 239.30321 | 20.03754 | 0.04943 | $616 \pm 75$ | $1.5 \pm 0.2$ | $14.6 \pm 0.2$ | -1.84 | N | 0.250 (2/8) |
| Cluster1558+18 | 239.58604 | 18.08087 | 0.04555 | $473 \pm 56$ | $1.1 \pm 0.1$ | $14.3 \pm 0.2$ | -1.08 | N | 0.182 (2/11) |
| Cluster1602+16 | 240.68797 | 16.24820 | 0.03522 | $985 \pm 79$ | $2.4 \pm 0.2$ | $15.2 \pm 0.1$ | -4.10 | Y: Substructure | 0.329 (25/76) |
| Cluster1604+23 | 241.23463 | 23.75779 | 0.03123 | $347 \pm 47$ | $0.8 \pm 0.1$ | $13.9 \pm 0.2$ | -2.18 | N | 0.714 (5/7) |
| Cluster1605+17[b] | 241.34383 | 17.85508 | 0.03613 | $786 \pm 60$ | $1.9 \pm 0.1$ | $14.9 \pm 0.1$ | -5.00 | Y: Substructure | 0.438 (14/32) |
| Cluster1611+29 | 242.93950 | 29.73384 | 0.04987 | $516 \pm 63$ | $1.2 \pm 0.2$ | $14.4 \pm 0.2$ | -0.12 | Y: Pair | 0.667 (2/3) |
| Cluster1613+30 | 243.28699 | 30.82703 | 0.05106 | $660 \pm 77$ | $1.6 \pm 0.2$ | $14.7 \pm 0.2$ | -0.27 | Y: Pair | 0.333 (3/9) |
| Cluster1613+49 | 243.32796 | 49.10888 | 0.05768 | $490 \pm 54$ | $1.2 \pm 0.1$ | $14.3 \pm 0.2$ | -2.33 | N | 0.250 (3/12) |
| Cluster1617+35 | 244.39828 | 35.13410 | 0.03226 | $573 \pm 60$ | $1.4 \pm 0.1$ | $14.5 \pm 0.1$ | -0.63 | N | 0.312 (5/16) |
| Cluster1627+14 | 246.90915 | 14.01201 | 0.05180 | $375 \pm 44$ | $0.9 \pm 0.1$ | $13.9 \pm 0.2$ | -2.36 | N | 0.091 (1/11) |
| Cluster1628+40 | 247.22563 | 40.86662 | 0.03034 | $587 \pm 42$ | $1.4 \pm 0.1$ | $14.5 \pm 0.1$ | -4.22 | Y: Substructure | 0.486 (17/35) |
| Cluster1629+39 | 247.49731 | 39.52851 | 0.02891 | $751 \pm 64$ | $1.8 \pm 0.2$ | $14.9 \pm 0.1$ | -0.03 | Y: Pair | 0.432 (16/37) |
| Cluster1631+13 | 247.99683 | 13.60695 | 0.05256 | $449 \pm 50$ | $1.1 \pm 0.1$ | $14.2 \pm 0.2$ | -0.44 | N | 0.286 (4/14) |
| Cluster1633+11 | 248.40599 | 11.88226 | 0.05190 | $399 \pm 55$ | $1.0 \pm 0.1$ | $14.0 \pm 0.2$ | -0.54 | N | 0.100 (1/10) |
| Cluster1650+23 | 252.72729 | 23.30994 | 0.03585 | $486 \pm 69$ | $1.2 \pm 0.2$ | $14.3 \pm 0.2$ | -0.89 | N | 0.500 (2/4) |
| Cluster1654+23 | 253.62039 | 23.41564 | 0.05582 | $475 \pm 74$ | $1.1 \pm 0.2$ | $14.3 \pm 0.2$ | -0.09 | N | 0.250 (2/8) |
| Cluster1714+57 | 258.65015 | 57.49308 | 0.02935 | $638 \pm 88$ | $1.6 \pm 0.2$ | $14.6 \pm 0.2$ | -0.42 | N | 0.333 (3/9) |
| Cluster2142−06 | 325.69135 | -6.86461 | 0.05153 | $545 \pm 52$ | $1.3 \pm 0.1$ | $14.4 \pm 0.1$ | -0.31 | N | 0.300 (3/10) |
| Cluster2157−07 | 329.33923 | -7.81302 | 0.05866 | $597 \pm 48$ | $1.4 \pm 0.1$ | $14.6 \pm 0.1$ | -2.59 | N | 0.200 (5/25) |
| Cluster2215+13 | 333.87616 | 13.67317 | 0.02505 | $363 \pm 68$ | $0.9 \pm 0.2$ | $13.9 \pm 0.3$ | -0.08 | N | 0.250 (1/4) |

*Supplementary Table 1 continued on next page*

**Supplementary Table 1** *(continued)*

| Name | RA | Dec | Redshift | $\sigma_v$ [km s$^{-1}$] | $R_{200}$ [Mpc] | $\log(M_{200}/M_\odot)$ | $\log p$ | Interacting | $f_{\rm bar}$(bar/disk) |
|---|---|---|---|---|---|---|---|---|---|
| (1) | (2) | (3) | (4) | (5) | (6) | (7) | (8) | (9) | (10) |
| Cluster2243+00 | 340.84122 | 0.33859 | 0.05932 | $395 \pm 53$ | $1.0 \pm 0.1$ | $14.0 \pm 0.2$ | -0.61 | N | 0.000 (0/3) |
| Cluster2324+14 | 351.15302 | 14.61110 | 0.04136 | $641 \pm 69$ | $1.6 \pm 0.2$ | $14.7 \pm 0.1$ | -0.44 | N | 0.200 (2/10) |

NOTE—Column 1: names of clusters in this study. Column 2 & Column 3: right ascensions and declinations of clusters. Column 4: redshifts of clusters. Column 5: velocity dispersions of clusters in unit of km s$^{-1}$. The errors were calculated by random sampling (10,000 times) of cluster members. Column 6: $R_{200}$ of clusters in unit of Mpc, where $R_{200}$ is the radius within which the mean density is 200 times the critical density of the universe. The errors were computed by random sampling (10,000 times) of cluster members. Column 7: logarithmic value of $M_{200}$ of clusters, where $M_{200}$ is cluster mass in $R_{200}$. The errors were derived by random sampling (10,000 times) of cluster members. Column 8: logarithmic $p$ values of clusters which indicate significance of having substructure. The small $p$-value (or the large $1 - p$-value) denotes high probability of existence of substructures in a cluster. Column 9: clusters that were classified as interacting ones are marked as Y. In these cases, we also mark whether clusters are in pairs or have substructures. Otherwise, N is marked in this column. Column 10: bar fractions of clusters. We also show the numbers of disk galaxies with $e$(ellipticity) $\leq 0.5$ and B/T (bulge-to-total light ratio) $\leq 0.5$ in each cluster as well as the numbers of barred galaxies among them.

[a] We found that Cluster1132+55 is a combination of two clusters having $\log(M_{200}/M_\odot) \sim 14.0$ and $\log(M_{200}/M_\odot) \sim 14.6$–15.0 that are overlapped in the line of sight with the peak separation of $\sim 2200$ km s$^{-1}$ in the velocity space. However, in our analysis, we regard Cluster1132+55 as a single cluster of $\log(M_{200}/M_\odot) = 15.3$ with two different peaks (or redshifts) in the velocity space, due to the difficulty of separating the cluster into individual clusters.

[b] The $p$-value of Cluster1605+17 was found to be 0. So we set the $p$-value to be $10^{-5}$ as an upper limit.

## SUPPLEMENTARY REFERENCES


1. Lin, Y.-T., Mohr, J. J. & Stanford, S. A. K-band properties of galaxy clusters and groups: luminosity function, radial distribution, and halo occupation number. *Astrophys. J.* **610**, 745-761 (2004).
2. Muzzin, A., Yee, H. K. C., Hall, P. B., Ellingson, E., & Lin, H. Near-infrared properties of moderate-redshift galaxy clusters: luminosity functions and density profiles. *Astrophys. J.* **659**, 1106-1124 (2007).
3. Budzynski, J. M., Koposov, S. E., McCarthy, I. G., McGee, S. L. & Belokurov, V. The radial distribution of galaxies in groups and clusters. *Mon. Not. R. Astron. Soc.* **423**, 104-121 (2012).
